# Supplementary material for: MuViSeg: Multi-View Segment Correspondences from Dense Geometry Priors
Source: arXiv:2607.17938 source file (2026-10-03)
Supplement: Supplementary file 1 [file supplementary.tex]

\clearpage
\appendix
\section*{Supplementary Material}
\setcounter{section}{0}

\setcounter{figure}{0}

\section{Multi-view sweep: effect of $N$} \label{app:nsweep}

Figure~\ref{fig:nsweep} plots the Joint model at $N \in \{2, 4, 6, 8\}$ per angular bin (trained with $N{=}4$, evaluated at each $N$ without retraining). On Replica $N$ has almost no effect ($81.10$--$81.57$ overall AUPRC): indoor scenes have dense per-view overlap, so extra views add little. On Virtual KITTI~2, $N$ helps specifically at wide baselines: the $135$--$180^\circ$ bin improves from $71.05$ ($N{=}2$) to $78.22$ ($N{=}6$) before saturating, while narrow bins stay flat around $47.5\%$ --- a per-pair VGGT bottleneck that adding views cannot solve. The model extrapolates to $N = 6, 8$ without collapse even though the position-embedding indices $4$--$7$ are never directly supervised, consistent with joint attention learning view-relative rather than view-absolute patterns.

\begin{figure}[h]
  \centering
  \includegraphics[width=\linewidth]{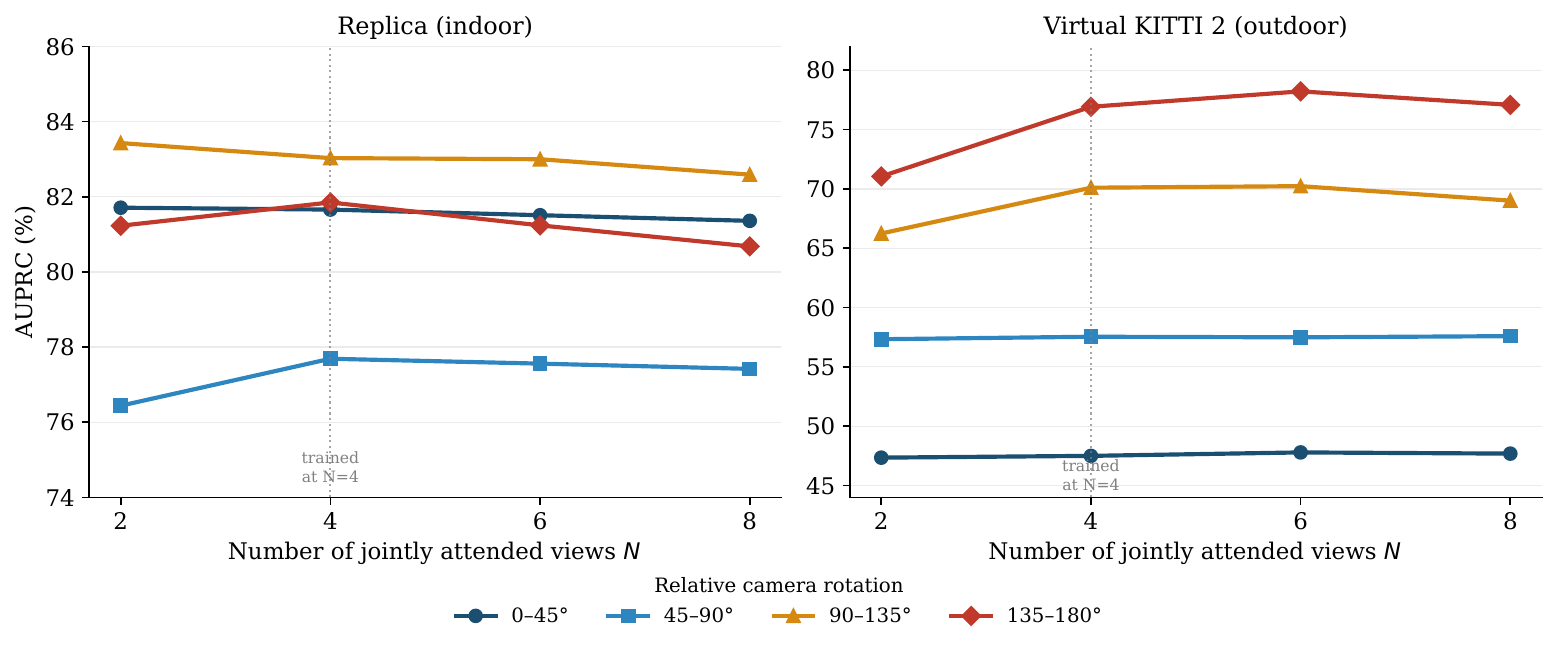}
  \caption{Effect of the number of jointly attended views $N$ on SegVGGT-DPT Joint (trained at $N{=}4$, evaluated at $N\in\{2,4,6,8\}$ without retraining). Replica (left) is flat in $N$ (dense overlap); on VKITTI2 (right) extra views help only at the widest baseline ($71.1{\to}78.2$ AUPRC at $135$--$180^\circ$) and saturate by $N{=}6$.}
  \label{fig:nsweep}
\end{figure}

\section{Ablation: temperature clamping} \label{app:tempclamp}

The DoubleSoftmax temperature $\tau$ is learned for the VGGT heads (Section~\ref{sec:method}), and we found its calibration to be the binding constraint on SegVGGT-DPT's accuracy. To see why clamping it to $\tau \le 1.0$ matters, we decompose the head's failures into three mutually exclusive types and count how the error budget is spent: \emph{false-dustbin} (a true correspondence wrongly sent to the dustbin, \ie{} the head abstains when it should match), \emph{wrong-match} (matched to the wrong segment), and \emph{false-match} (a spurious match for a segment that has no ground-truth counterpart). Figure~\ref{fig:errordecomp} plots the per-query error rate of each type, before and after clamping. Without clamping, an unbounded $\tau$ over-sharpens the score distribution, so the head becomes over-confident about abstaining: \emph{false-dustbin} dominates the error budget and the model discards true correspondences. Clamping $\tau \le 1.0$ (with matchability weight $\lambda{=}0.3$) cuts the \emph{false-dustbin} rate by $36\%$ relative and re-allocates the residual budget toward the genuinely harder \emph{wrong-match}/\emph{false-match} cases. The takeaway is that for this head calibrated scoring, not richer descriptors, is what limits accuracy.

\begin{figure}[h]
  \centering
  \includegraphics[width=0.72\linewidth]{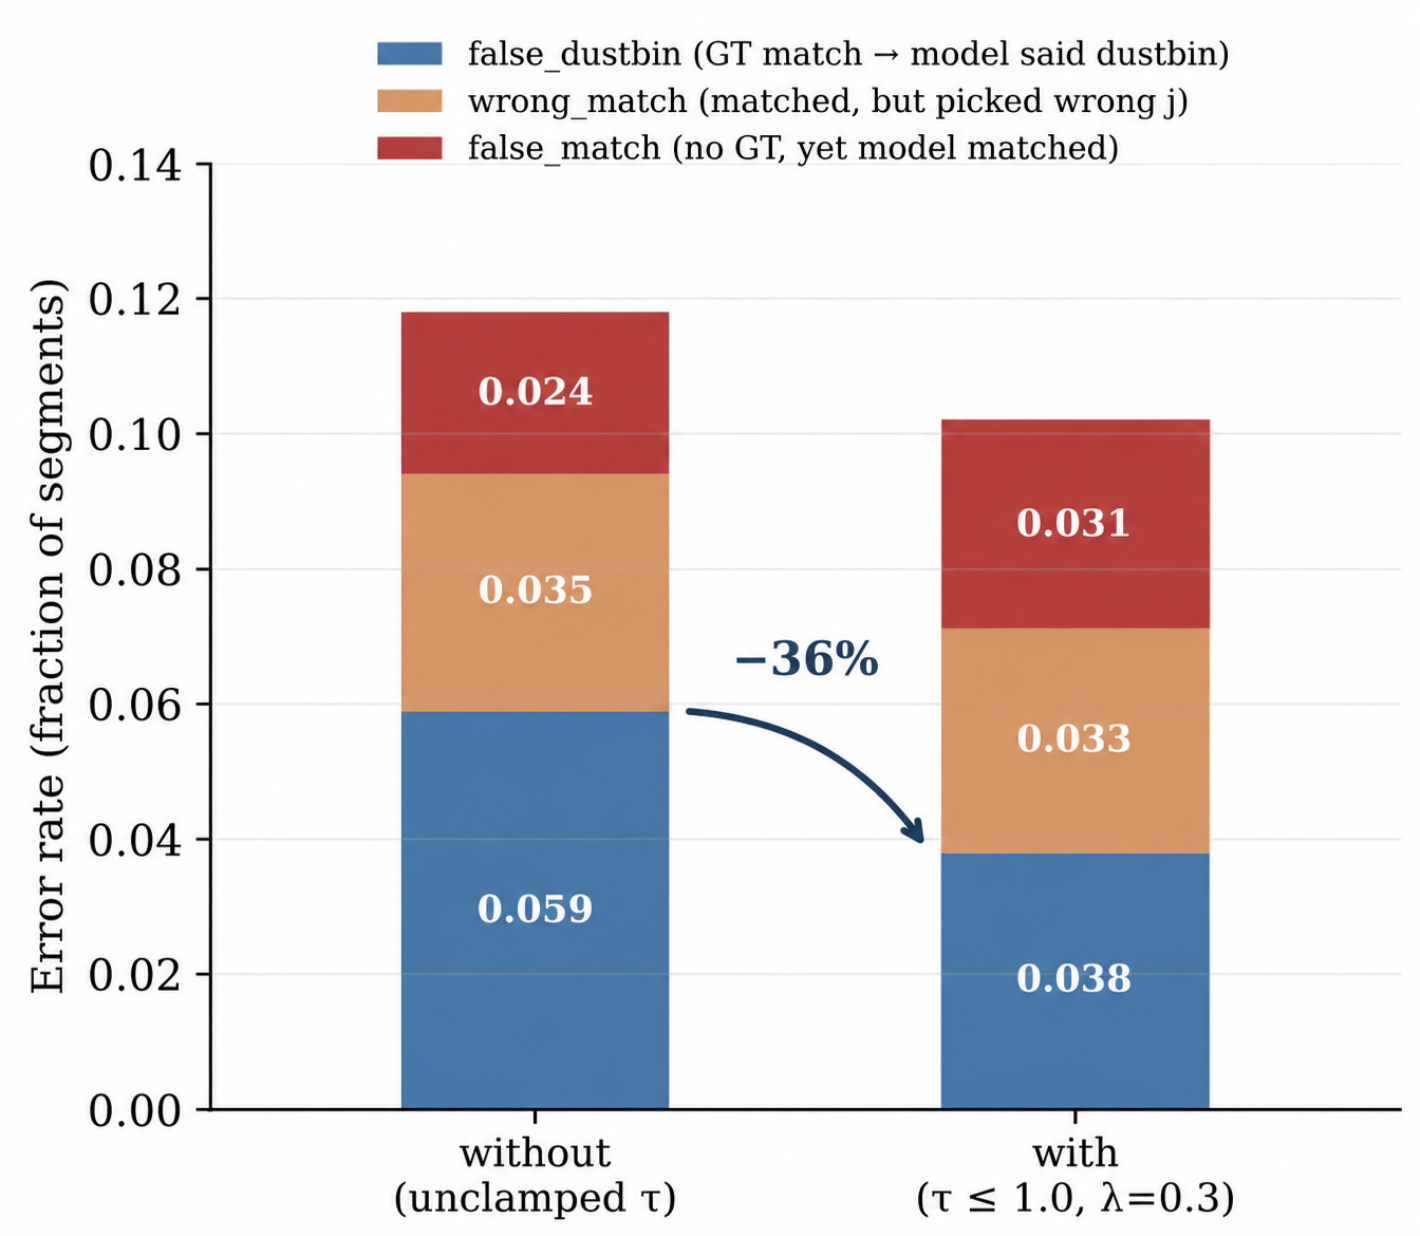}
  \caption{Temperature-clamp ablation on SegVGGT-DPT: per-query error rate by failure type, before (left) and after (right) clamping $\tau \le 1.0$ ($\lambda{=}0.3$). Clamping cuts the dominant \emph{false-dustbin} errors by $36\%$ relative, shifting the residual budget to the harder \emph{wrong-match}/\emph{false-match} types.}
  \label{fig:errordecomp}
\end{figure}
